# Supplementary material for: An Incremental Algorithm for Algebraic Program Analysis
Source: arXiv:2412.10632 source file (2024-12-14)
Supplement: Supplementary file 2 [file 0_appendix_main.tex]

\clearpage
	% \onecolumn
	\appendix

% 

% \tableofcontents

\subsection{Left-over Materials \textcolor{red}{(moved from the ``Experiments'' section by Chao)}}

We only take the action of change, which means change the interpretation or connection of one single node. The reason why we first research this option is that it will not influence the graph's size, and can model many kinds of modifications or changes in real world. Here we give the formal definition of each modification options:

\begin{itemize}
    \item \textbf{Change($u,val$)}. It changes the node $u$'s value into $val$. Here $u$ is the node(a dataflow transformation function in our experiment), and $value$ is the new value of node $u$. 
    \item \textbf{Insert($u, v, w$)}. It inserts a node $w$ between nodes $(u, v)$. Here including the nodes $v$ to make the location more precise. 
    \item \textbf{Delete($u$)}. It deletes a node $u$ from the graph.
\end{itemize}

The delete option is a little bit tricky here. In a easiest way, we can just change the value to $ZERO$, so it will have the same effect. However, it has a potential drawback that it will increase the actual size of the graph, makes the time cost larger. Here we still use the Scapegoat strategy, we will keep use the `lazy' strategy by changing the node's value to $ZERO$, it is the same as marking a node as deleted. We also maintain a rebalance fraction $\theta=\frac{n_{\text{deleted nodes}}}{n_{\text{all nodes}}}$ for each node,  Each time of query and insert, when we found the rebalence fraction is greater than some bound, we will start a cleaning process and delete all the marked deleted nodes.

In our experiments, we choose some function and do the modification many time. Though the preprocess of DeComp may be relatively fast, but when the query time increases, the total query time is still not acceptable. For the Tarjan Algorithm, 
each time they will only need to recalculate the dominate tree and the graph information, the DeComp algorithm need to redo the inter and intra procedural preprocess.

\textbf{Tree building}. In tree building process, there are mainly two steps: calculating the tree expression and updating the tree node information. Our APA-Tree is actually an interval tree, means that each node of the tree is a set of actual node of original graph. In traditional 1D situation, people use the endpoints of intervals to locate the actual node's position in the tree. But in our settings, the tree is built based on expression tree, so it is hard to locate base on interval endpoints. Here we use a hash map to record which actual node is contained in the subtree. According to the graph, maintaining the hash table is the most time-consuming part due to the complexity of hash table merging. This part can be improved in the future if split the nodes more precisely, so the time consuming can be furtuer reduced. 

\textbf{Tree querying}. In the tree querying process, there are also two steps: locating the node and update the information. As previously introduced, both parts are related to the location technique. In our current selection, as the locating only involves hash table query, it is relatively faster than updating the new hash table. Here besides the previously mentioned endpoint based improvement, an incremental update of hash table can also be considered to accelerate this process. 

\subsection{Types of Program Changes}

The word `incremental' means that we can make some updates on a original analyzed program, and expecting the analyzer to calculate the new analysis result quickly. Here we assume every incremental change will only have the budget of modifying only one statement in the original program. It is obvious that any more complex increments can be decomposed into such smaller changes. Based on that, we can separate the incremental changes into two category:

\begin{itemize}
    \item \textbf{Non-structural Increments}. Some changes like modifying the branch condition expression, modifying the content of assignment expression will not influence the topological structure of CFGs. 
    \item \textbf{Structural Increments}. Some changes like inserting control statements like continue, break, or inserting new branches and loops will influence the CFG's structure.
\end{itemize}

These two kinds of increments has different difficulties for APA. For efficiently handles these kinds of queries, we have three atomic operations for APA:

\begin{itemize}
    \item \textbf{Change($u,val$)}. It changes the node $u$'s value into $val$. Here $u$ is the node(a dataflow transformation function in our experiment), and $value$ is the new value of node $u$. 
    \item \textbf{Insert($u, v, w, W$)}. It inserts a node $w$ between nodes $(u, v)$. Here including the nodes $v$ to make the location more precise. The $W$ is a set of nodes indicating which new nodes the $w$ will connnect to. 
    \item \textbf{Delete($u$)}. It deletes a node $u$ from the graph.
\end{itemize}

\subsubsection{Non-structural Increments}

The non-structural increments can be directly mapped to change operations. Here in traditional algebraic program analysis, these change will not influence the path expression, but only regard to the path interpretation. Since will still need to reinterpret the whole path expression, these changes will only change the interpretation stage.

\subsubsection{Structural Increments}

Here we want to discuss how to model some common control flow changes into these atomic operations. Generally speaking, we will the following kinds of statements which will potentially influence the CFG structure.

\textbf{Branches and Loops}

Branches and loops generally divided into two steps: inserting new nodes and changing the connection of nodes. Inserting new branch nodes will automatically have new connection relationship, and loops are little bit tricky as we need to modify the loop body end node's connection. It can be achieved by simple deleting it and adding it again with new connections. 

\textbf{Loop Halting}

Loop halting statements will break the original loop structure. To minimize the influence of these statements on graph, we have the following modifications:

\begin{itemize}
    \item Before handling the program, we will start a program rewrite to rewrite every loop into single entry-single out. For original and newly inserted `break' statements, we will translate it into combination of `if' and `continue'. They are equivalent in semantic.
    \item For the new `continue' statements, the influence on the program can be modeled as ~\autoref{fig:insert_continue}. Generally it will insert a new node and make it connect to the loop starting node.
\end{itemize}

\begin{figure}[htbp]
    \centering
    \includegraphics[width=1\linewidth]{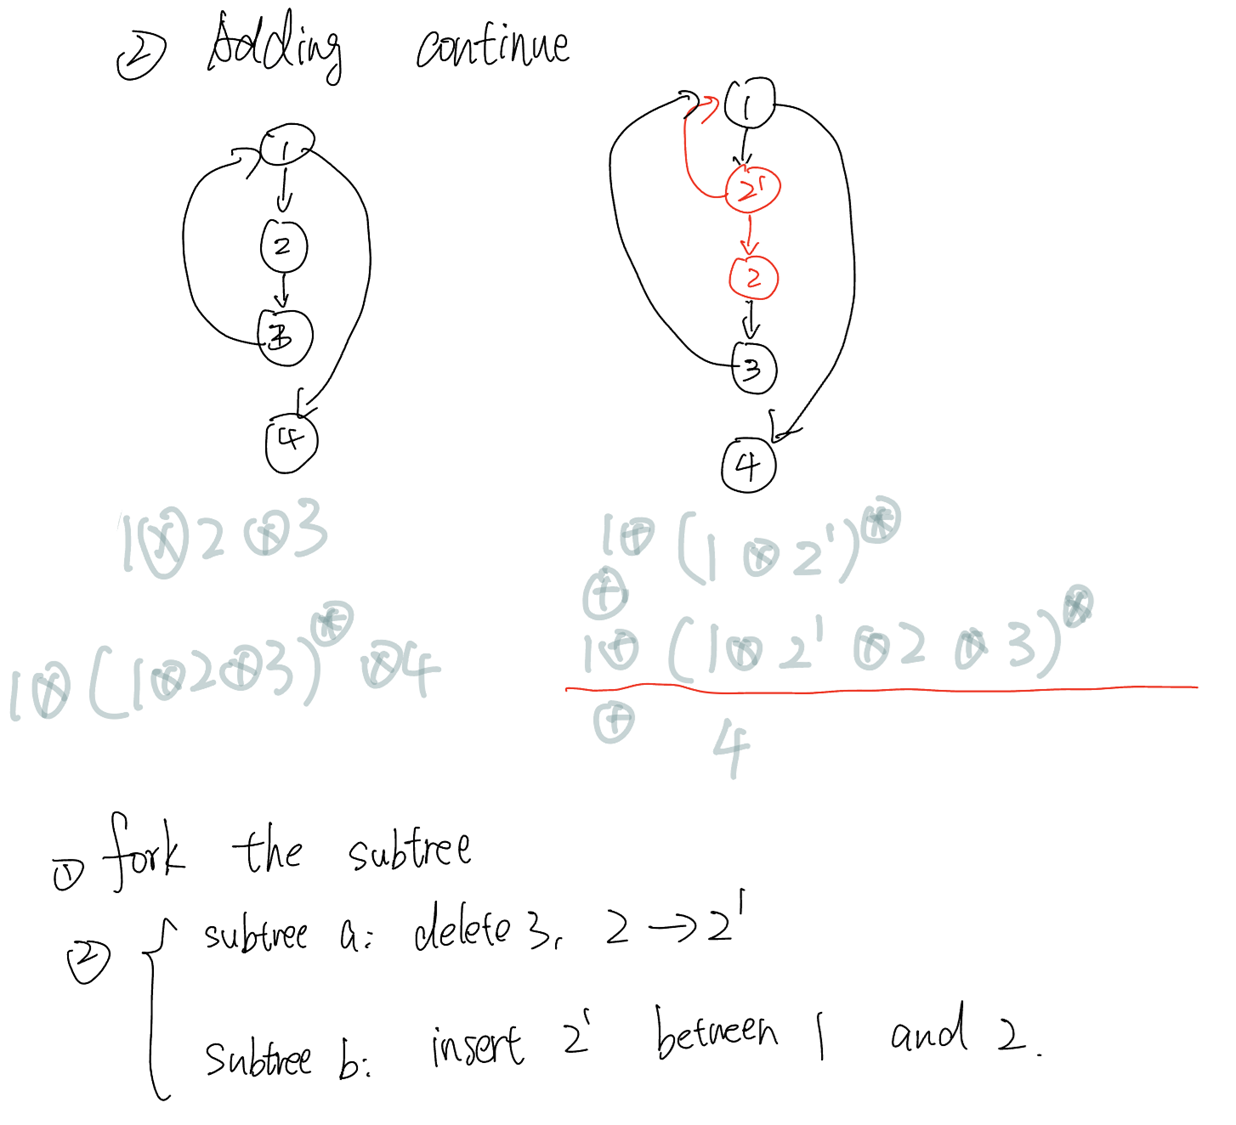}
    \caption{Inserting new 'continue' into a program-\red{UNFINISHED}}
    \label{fig:insert_continue}
\end{figure}

After designing the options to the graph, we can further handle these operations on our APA-Tree structure.

% The structural increments will directly influence the path expression for APA, which we want to maintain incrementally. 

% \textbf{Insert($u, v, w$)}. For the insert operation, we will find the target leaf node $u$. Since our APA-Tree is maintains intervals, we will make two new child nodes valued $u, v$ as its new child nodes, and update the original node as the union of these two nodes. By doing this, we will not violate the property of trees. However, inserting too much may cause the imbalance of the tree. We will discuss how to handle this issue later.

% \textbf{Delete($u$)}. The deleting operation is a little bit tricky here. 
